# Supplementary material for: Physical Properties and Thermal Stability of Zirconium Platinum Nitride Thin Films
Source: arXiv:2407.17653 ancillary file (2024-07-24)
Supplement: Supplementary file 1 [file supplementary.pdf]

# **Supplementary Material: Physical Properties and Thermal Stability of Zirconium Platinum Nitride Thin Films**

R.A. Gallivan, A. Michelini, J. Manser, N. Toncich, N. Abando Beldarrain, and H. Galinski

*Laboratory for Nanometallurgy, Department of Materials, ETH Zurich*

C. Vockenhuber and A. Müller

*Ion Beam Physics, Department of Physics, ETH Zurich*

(\*henning.galinski@mat.ethz.ch)

(\*rebecca.gallivan@mat.ethz.ch)

(Dated: June 3, 2024)

## I. MATERIALS & METHODS

### A. Reactive Sputtering

The ZrN and ZrPt<sub>x</sub>N<sub>y</sub> film were deposited by reactive magnetron sputtering. The deposition was done at  $T = 400 - 450^\circ\text{C}$  at  $p = 3$  mTorr, 30 sccm argon flow, 3 sccm nitrogen flow. The base pressure was kept around  $10^{-7}$  mBar during all depositions. To ensure a uniform deposition the substrate was rotating with 20 rpm. The following targets were used: Zr, Pt, and an additional Zr target as oxygen gatherer. For the Zr-target a power of 300 W and for the Zr oxygen gatherer a power of 150 W was used. The power of the Pt target was varied between 0, 25, 50, and 75 W to adjust Pt content in the ZrPt<sub>x</sub>N<sub>y</sub> films. Depending on which measurement was performed with the sample, thin films were deposited either directly on Si-wafer pieces (for XRD, RBS, ERDA, and ellipsometry experiments) or on a glass slide for thickness calibration using an AFM (Witech alpha300 RA). The samples were annealed for 1 h in a vacuum at  $1 \times 10^{-9}$  mbar in a *Createc* rapid-thermal annealing (RTA) setup. The heating rate was kept at 2 K/min to avoid crack formation and no active cooling was used.

### B. Optical Characterization

To determine the refractive index of the ZrN and ZrPt<sub>x</sub>N<sub>y</sub> films an ellipsometer (J.A. Woollam M-2000) was used. The measurement was done at different angles from  $64^\circ - 72^\circ$ . For the ellipsometric measurements, the 120 nm ZrN and ZrPt<sub>x</sub>N<sub>y</sub> samples were deposited on glass slides. The ZrN sample was fitted with the Au model because ZrN exhibits similar optical properties to Au. For the further measurements of the Pt-containing samples, a fitting model based on the first measured ZrN values was used. To get more insight into how the addition of Pt alters the optical response, we have fitted the measured optical properties with a Drude-Lorentz model using the software RefFit[2]. Using the Drude-Lorentz model we can treat the optical response as a sum of separate resonances. These resonances are typically due to several phenomena such as lattice vibrations, ionic oscillations, and oscillations of free and bound electrons. The Drude-Lorentz formula reads

$$\varepsilon(\omega) = \varepsilon_\infty + \frac{\omega_p^2}{\omega^2 - i\gamma\omega} + \sum_i \frac{\omega_i^2}{\omega_{0i}^2 - \omega^2 - i\gamma_i\omega}, \quad (1)$$

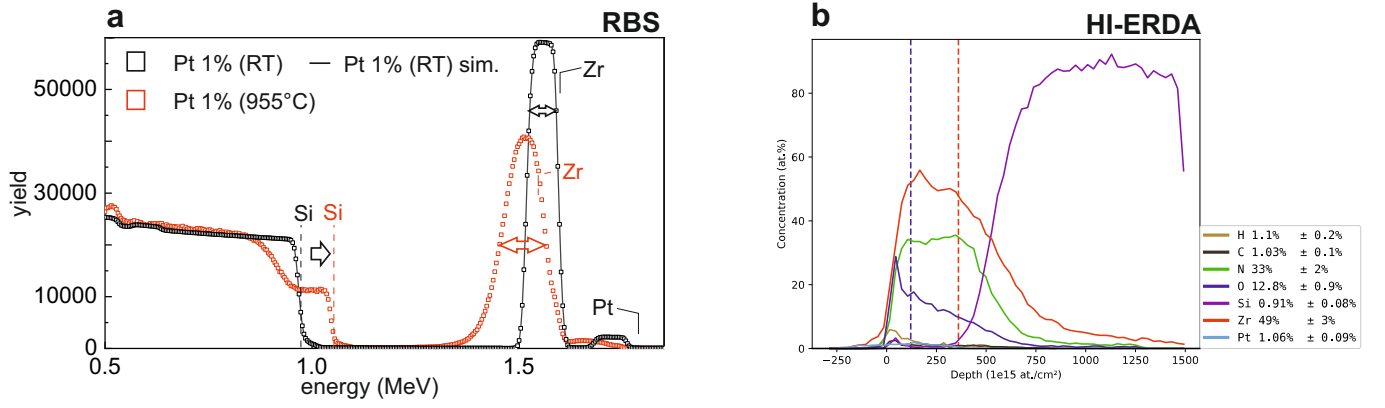

Figure 1. (a) Comparison of RBS spectra ZrN + Pt 1% at RT and after annealing at 955 °C for 1 h. The RBS measurements were conducted with a 2 MeV He beam under a scattering angle of 167.5°. The observed shift of the Si-edge and the broadening of the Zr-peak is indicative of a solid state reaction, in agreement with XRD and SEM data. (b) Representative HI-ERDA depth profile of ZrN + Pt 1%. The ERDA spectra were analyzed with the Potku software [1] and depth profiles have been created for light elements and Zr and Pt. The measurements were obtained using a 13.6 MeV iodine beam hitting the sample under a angle 18° relative to the sample surface. The elemental composition was determined only in the depth region between the dashed blue and red markers.

whereby  $\epsilon_\infty$  is the high-frequency dielectric constant in ( $\text{cm}^{-1}$ ),  $\omega_{0i}$  designates the transverse frequency of the  $i$ -th oscillator,  $\omega_p, \gamma$  are the plasma frequency and scattering rate of the Drude term, while  $\omega_i$  is the central frequency and  $\gamma_i$  the scattering rate of the  $i$ -th Lorentz term. Of particular importance is the screened plasma frequency  $\omega_p$  in the Drude term as it is directly proportional to the total free carrier concentration  $n$ . To include the screening effects within the materials, often the screened the plasma frequency  $\tilde{\omega}_p$  is used, which is given by

$$\tilde{\omega}_p = \sqrt{\frac{ne^2}{m^* \epsilon_\infty}}, \quad (2)$$

where  $m^*$  is the effective electron mass of electrons in the conduction band.  $\tilde{\omega}_p$  takes on the role of a cut-off frequency, electromagnetic waves with  $\omega < \tilde{\omega}_p$  cannot propagate in the material and will be reflected.

### C. Beam-based Characterization

XRD scans were taken with a Panalytical X'Pert PRO MPD device with a scan range angle from 25 to 75. As a reference, an empty  $\text{SiN}_3$  was measured with a scan range angle from 5° to 80°. The thickness and stoichiometric composition between Zr and Pt in  $\text{ZrPt}_x\text{N}_y$  was determined with RBS (SFigure 1a). The data was received by 2 MeV He RBS. No tilt was applied to the samples. The solid lines in the data curves come from RUMP simulations; the points represent the actual measured data. 13 MeV  $^{127}\text{I}$  Heavy Ion ERDA was used to determine the oxygen and nitrogen content in the  $\text{ZrPt}_x\text{N}_y$  (SFigure 1b). The mass spectra of the center part of the film have been extracted and C/N/O ratios have been determined. The ERDA spectra were analyzed with the Potku software and depth profiles have been created.

### D. Nanoindentation Methods

Using an iNano nanoindenter (Nanomechanics, Inc.) with an InForce50 actuator, all samples were indented to a load of 1 mN using a diamond Berkovich tip (Synton-MDP). The indentation load was determined by performing indents from 0.1 – 2 mN and selecting a load within the regime where hardness does not depend on indentation depth for all samples.

Indents were performed using the NanoBlitz<sup>TM</sup> program in a square grid of 50 x 50 indents. This method provides strong statistical insight into the measured hardness and highlights any spatial variation in hardness. All hardness and modulus measurements are reported at the maximum indentation depth.

### E. DFT calculations

We employ DFT calculations using the Quantum ESPRESSO package [3] in the generalized gradient approximation for the exchange-correlation functional as parametrized by Perdew, Burke, and Ernzerhof (PBE) [4]. The primitive cells contained 2 (ZrN) and 28 atoms (ZrPtN), respectively. Atomic positions are fully relaxed until all force components are smaller than 0.1 mRy/ $a_0$  ( $a_0$  : Bohr radius) and the cell volume is relaxed until all components of the stress tensor remain under 0.5 kbar. The kinetic energy cut-off was determined by minimizing the total energy difference and was set to 45 Ry. Structural relaxation of  $\text{Zr}_2\text{PtN}$ ,  $\text{Zr}_{16}\text{Pt}_6\text{N}_6$  was realized by substituting N for Pt

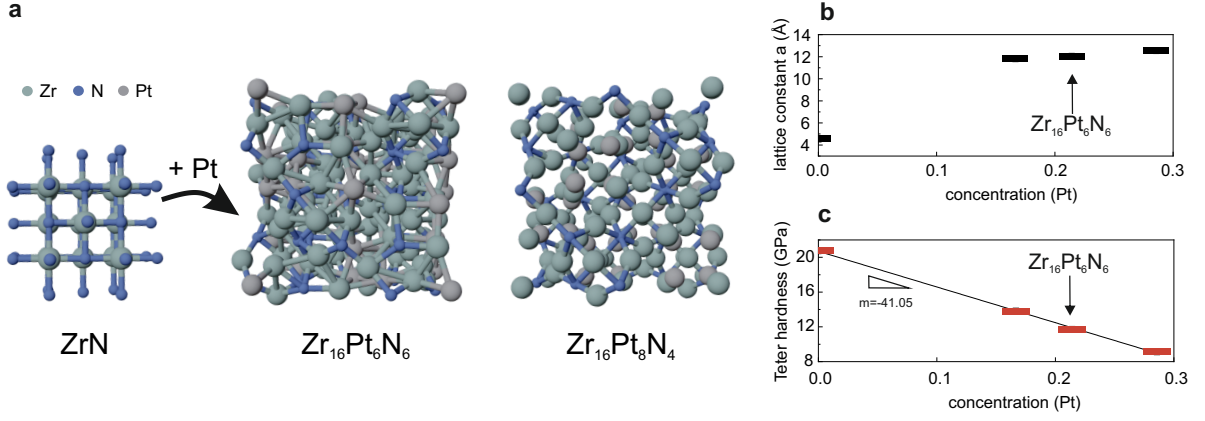

SFigure 2. DFT calculations using Quantum ESPRESSO (a) Relaxed geometries of ZrN, Zr<sub>16</sub>Pt<sub>6</sub>N<sub>6</sub>, Zr<sub>16</sub>Pt<sub>8</sub>N<sub>4</sub> obtained after full relaxation without symmetry constraints. All structures exhibit cubic symmetry. Pt substitutes N on the non-metallic sublattice which is consistent with the experiment. (b) Simulated lattice parameter, *a*, of the conventional cells as function of Pt-content for four modeled ZrN-based materials, namely ZrN, Zr<sub>2</sub>PtN, Zr<sub>16</sub>Pt<sub>6</sub>N<sub>6</sub>, and Zr<sub>16</sub>Pt<sub>8</sub>N<sub>4</sub> (c) Teter hardness, *H<sub>v</sub>*, plotted as function of Pt-content for four modeled ZrN-based materials, namely ZrN, Zr<sub>2</sub>PtN, Zr<sub>16</sub>Pt<sub>6</sub>N<sub>6</sub>, and Zr<sub>16</sub>Pt<sub>8</sub>N<sub>4</sub>. A linear regression with *m* = −41.05 and *b* = 20.69 is fitted as guide for the eye.

in the geometry optimized Zr<sub>16</sub>Pt<sub>8</sub>N<sub>4</sub> taken from Ref [5]. XRD spectra of each relaxed structure was achieved by using VESTA (RIETAN-FP). The electronic and thermomechanical properties of the relaxed structures were estimated using AFLOW-ML [6].

SFigure 2a shows the calculated relaxed geometries of ZrN, Zr<sub>16</sub>Pt<sub>6</sub>N<sub>6</sub>, Zr<sub>16</sub>Pt<sub>8</sub>N<sub>4</sub>. All geometries are cubic and face-centered, but addition of Pt leads to threefold expansion of the unit cell (SFigure 2b). While ZrN forms a NaCl-like structure, addition of Pt leads to a transition in the crystallography, and a diamond-like structure is formed. The shear moduli *G* of the optimized geometries were estimated using AFLOW-ML [6]. Using the Teter approximation  $H_v = 0.151G$ , we calculated the hardness *H<sub>v</sub>* as function of Pt-content (SFigure 2c). Interestingly, the Teter hardness exhibits an overall linear scaling as a function of Pt-content, which might be due to the lack of data points for low Pt concentrations. SFigure 3 reports the calculated density of states for ZrN and Zr<sub>16</sub>Pt<sub>6</sub>N<sub>6</sub>, respectively. The results on ZrN are in good agreement with DFT calculations from literature [7, 8]. Here, the observed near-zero value of the DOS (ZrN=3.0 eV and Zr<sub>16</sub>Pt<sub>6</sub>N<sub>6</sub>= 6.6 eV) can be used to approximate the threshold energy of the interband transitions [8], which are comparable with measured reduced plasma frequency of the system.

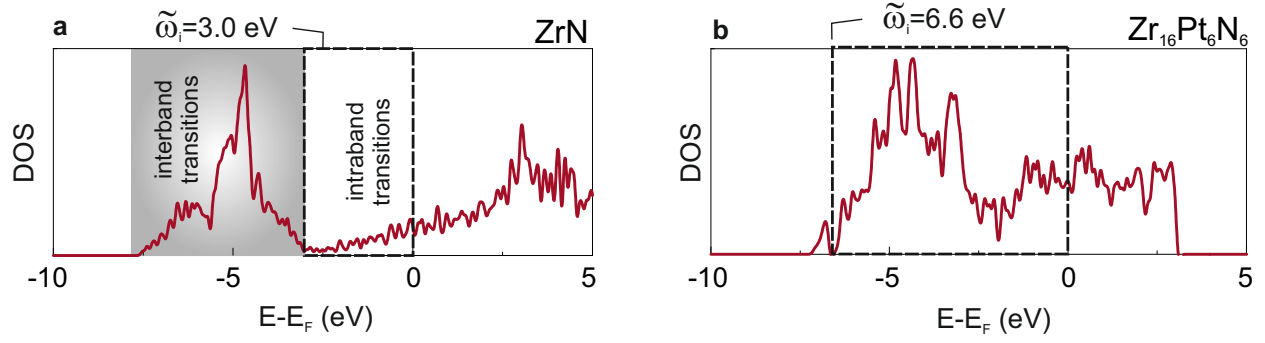

Figure 3. DFT calculations using Quantum ESPRESSO (a) Total density of states (DOS) of ZrN. Grey shaded region highlights the region where interband transitions from N-p to Zr-d levels dominate the optical response, while above the transition frequency  $\tilde{\omega}_i$  intraband transitions dominate the response. (b) DOS of  $\text{Zr}_{16}\text{Pt}_6\text{N}_6$ , the transition frequency  $\tilde{\omega}_i$  is shifted further to the UV upto a near-zero value of the DOS and the band edge.

- 
- [1] K. Arstila, J. Julin, M. Laitinen, J. Aalto, T. Konu, S. Kärkkäinen, S. Rahkonen, M. Raunio, J. Itkonen, J.-P. Santanen, T. Tuovinen, and T. Sajavaara, Nuclear Instruments and Methods in Physics Research Section B: Beam Interactions with Materials and Atoms **331**, 34 (2014), 11th European Conference on Accelerators in Applied Research and Technology.
  - [2] A. B. Kuzmenko, Review of Scientific Instruments **76**, 083108 (2005), [https://pubs.aip.org/aip/rsi/article-pdf/doi/10.1063/1.1979470/16127359/083108\\_1\\_online.pdf](https://pubs.aip.org/aip/rsi/article-pdf/doi/10.1063/1.1979470/16127359/083108_1_online.pdf).
  - [3] P. Giannozzi, S. Baroni, N. Bonini, M. Calandra, R. Car, C. Cavazzoni, D. Ceresoli, G. L. Chiarotti, M. Cococcioni, I. Dabo, A. Dal Corso, S. De Gironcoli, S. Fabris, G. Fratesi, R. Gebauer, U. Gerstmann, C. Gougoussis, A. Kokalj, M. Lazzeri, L. Martin-Samos, N. Marzari, F. Mauri, R. Mazzarello, S. Paolini, A. Pasquarello, L. Paulatto, C. Sbraccia, S. Scandolo, G. Sclauzero, A. P. Seitsonen, A. Smogunov, P. Umari, and R. M. Wentzcovitch, Journal of Physics Condensed Matter **21** (2009), 10.1088/0953-8984/21/39/395502.
  - [4] J. P. Perdew, K. Burke, and M. Ernzerhof, Physical Review Letters **77**, 3865 (1996).
  - [5] <https://aflow.org/material/?id=aflow:2fb74561ffd344ed>, <https://aflow.org/material/?id=aflow:2fb74561ffd344ed>.
  - [6] E. Gossett, C. Toher, C. Oses, O. Isayev, F. Legrain, F. Rose, E. Zurek, J. Carrete, N. Mingo, A. Tropsha, and S. Curtarolo, Computational Materials Science **152**, 134 (2018).

- [7] A. Shabani, M. Tsegay Korsas, S. Petersen, M. Khazaei Nezhad, Y. Kumar Mishra, and J. Adam, *Advanced Photonics Research* **2**, 2100178 (2021), <https://onlinelibrary.wiley.com/doi/pdf/10.1002/adpr.202100178>.
- [8] M. Kumar, S. Ishii, N. Umezawa, and T. Nagao, *Opt. Mater. Express* **6**, 29 (2016).
